# Supplementary material for: Rank2Reward: Learning Shaped Reward Functions from Passive Video
Source: arXiv:2404.14735 source file (2024-04-23)
Supplement: Supplementary file 1 [file appendix.tex]

\appendix

\setcounter{section}{0}
\setcounter{figure}{0}

\def\centsect#1{\Large\centering#1}
\section*{\centsect{Supplementary Material}}

\section{Algorithm Pseudocode}

We present pseudocode for our algorithm below. Rank2Reward can be integrated with any off the shelf RL method. 

\begin{algorithm}[h]
\caption{Rank2Reward}
\label{alg:rank2reward}
\begin{algorithmic}[1]
    \STATE \textbf{Require:} Expert demonstration data $\D^e = \{\tau_k\}_{k=1}^N$
    \STATE Initialize policy $\pi$, empty replay buffer $\mathcal{D}_{\text{RB}}$
    \STATE Initialize utility function $\hat{u}_\theta$ and classifier $D_\theta$ functions for estimating rewards $\hat{r}(s)$.

    \STATE \textcolor{blue}{// Train the ranking function $\hat{u}_\theta$}
    \FOR{step $n$ in \{1, \dots, $N_{\text{ranking}}$\}}
        \STATE Sample pairs of states from each trajectory, $(s_{i}^k, s_{j}^k) \sim \tau_k$
        \STATE Learn $\hat{u}_\theta$ with batch $\{ (s_{t_1}, s_{t_2})_k \}_{k=1}^{bs}$ using \Cref{eq:BCEranking}
    \ENDFOR

    \STATE \textcolor{blue}{// Joint policy optimization and reward learning}
    \FOR{step $n$ in \{1, \dots, N\}}
        \STATE Collect transitions $\{\tau_l\}_{l=1}^M$ using current policy $\pi$, store in $\mathcal{D}_{\text{RB}}$
        \IF{$n\, \% \,\texttt{reward\_update\_frequency} == 0$}
            % \STATE \textcolor{blue}{// Update the classification function $D_\theta$}
            \STATE Sample batch of states from expert, $s_e \sim \D^e$
            \STATE Sample batch of states from replay buffer $s_{\pi} \sim \mathcal{D}_{\text{RB}}$ 
            \STATE Update $D_\theta$ to classify $s_e$ from $s_\pi$ with BCE. 
        \ENDIF
        % \STATE \textcolor{blue}{// Policy optimization}
        \STATE Sample batch of transitions $s_\pi$ from $\mathcal{D}_{\text{RB}}$
        \STATE Update $\pi$ using Equation (\ref{eq:finalobj})
    \ENDFOR
\end{algorithmic}
\end{algorithm}

\label{sec:asf}

\subsection{Implementation Details}
In all of our simulated environments, we render image frames that are used as the state space for estimating rewards, but for the reinforcement learning agent, we also include robot specific proprioception. To speed up learning, we leverage pretrained visual features from a recently proposed temporal feature learning method (R3M) \cite{nair_r3m_2022} as a frozen encoder for training both the reward function and the policy. We also find that incorporating mixup \cite{zhang2017mixup} and spectral normalization \cite{miyato18spectralnorm} for regularization is helpful as well for training our ranking, $\hat{u}_\theta$ and classifier networks $D_\phi(s)$.

For policy learning in simulation, we leverage a model-free reinforcement learning method for learning from images, DrQv2 \cite{yarats2021drqv2, yarats2021image}, and replace the default convolutional encoder with a frozen R3M module \cite{nair_r3m_2022}. 
%This leverages an actor-critic technique with data augmentation to enable efficient and performant image based learning. 
For learning in the real world, we likewise use a frozen R3M encoder \cite{nair_r3m_2022} and a data-efficient actor-critic technique \cite{smith2022walk, hiraoka2021dropout} that leverages dropout to regularize training, allowing for more updates per collected data point. We selected these algorithms since they are able to efficiently learn from camera images, but these can be replaced with any image-based reinforcement learning method. 

\section{Real-World Experiments Details}
\label{sec:a2append}

\subsection{Experiments Snapshots}
\begin{figure}[H]
    \centering
    \includegraphics[width=\linewidth]{figs/reach_strip.png}
    \vspace{-0.5cm}
    \caption{Reaching Task}
    \label{fig:reach_strip}
\end{figure}

\begin{figure}[H]
    \centering
    \includegraphics[width=\linewidth]{figs/push_strip.png}
    \vspace{-0.5cm}
    \caption{Pushing Task}
    \label{fig:push_strip}
\end{figure}

\begin{figure}[H]
    \centering
    \includegraphics[width=\linewidth]{figs/obst_push_strip.png}
    \vspace{-0.5cm}
    \caption{Pushing with Obstacle Task}
    \label{fig:obst_push_strip}
\end{figure}

\begin{figure}[H]
    \centering
    \includegraphics[width=\linewidth]{figs/open_strip.png}
    \vspace{-0.5cm}
    \caption{Drawer Opening Task}
    \label{fig:open_strip}
\end{figure}

\begin{figure}[H]
    \centering
    \includegraphics[width=\linewidth]{figs/sweep_strip.png}
    \vspace{-0.5cm}
    \caption{Sweeping Task}
    \label{fig:sweep_strip}
\end{figure}

\begin{figure}[H]
    \centering
    \includegraphics[width=\linewidth]{figs/draw_strip.png}
    \vspace{-0.5cm}
    \caption{Drawing Task}
    \label{fig:draw_strip}
\end{figure}

\subsection{Real-World Evaluation Metrics}
\label{sec:metrics}
For each task, we defined a metric to quantify the quality of learning across different agents. Although all metrics are evaluated by a human researcher, the metrics are designed to be as objective as possible. For reaching, we chose the $L2$-distance in centimeters (cm) between the end effector position and the target destination. Since the robot control interface does provide the real-time positions of the end effector, we use it to record the position of the target destination. When an evaluation episode ended, we applied the Euclidean distance formula to the positional data between the end effector of the xArm and the target. For pushing, we have a finish line where the expert data demonstrated to push the block over. At the end of an evaluation episode, we hand-measured the distance between the far end of the block and the finish line. If the distance is negative, i.e. the block is pushed over the line, we also record it as 0 as it accomplished the goal. For pushing with obstacle, we also set up a finish line over which the agent needs to push the block. However, it is more difficult to measure the results with distances because the agent can push the block over but hit the obstacle, which it should avoid. Therefore, we use a success/fail metric, where success means the agent needs to push the block over the finish line while not moving the obstacle during the process. We then record the minimum steps to successfully complete the task for each agent. For drawer opening, since the expert data only demonstrate to open the drawer and not how far out the drawer should be, we also use the success/fail system as metrics. The evaluation episode is counted as a success if the drawer is opened to more than half of its length, which is consistent across all expert data. We compared agents by the number of steps required for them to have a successful evaluation episode. For sweeping, we placed exactly 20 plastic beads each time at the beginning of an evaluation episode. We then counted the number of beads that are left on the table. The incompletion rate is thus given by $\frac{\text{number of beads left}}{20}$. We trained both agents until one of the agents reached 0\% incompletion, i.e. all beads on the table were swept off. We compare the agents by recording the incompletion rate in comparison to the other agent given the same amount of training. For the drawing task, we again use the success/fail system as our metric. The episode succeeds if an "L" shape can be reasonably recognized after the agent completes the drawing. 

\subsection{Hyperparameters Tables}
\begin{table}[H]
    \centering
    \begin{tabular}{| c || c |}
     \hline
     \textbf{METHOD} & \\
     \hline
     \textbf{DroQ}  & \\
     \hline
     action learning rate & $3 \times 10 ^{-4}$ \\
     critic learning rate & $3 \times 10 ^{-4}$ \\
     temperature learning rate & $3 \times 10 ^{-4}$ \\
     hidden dimensions & (256, 256) \\
     discount & 0.99 \\
     $\tau$ & 0.005 \\
     \# of Qs & 2 \\
     \hline
     \textbf{R3M} & \\
     \hline
      ResNet size & 18 \\
      embedding dimension & 512 \\
     \hline
     \textbf{Rank2Reward}(Ours) & \\
     \hline
     training batch size & 32 \\
     learning rate & $1 \times 10 ^{-4} $ \\
     hidden layers dimensions & (4096, 4096, 4096) \\
     non linearity & ReLU \\
     regularization on hidden layers & (None, None, Spectral Norm) \\
     ranking network training steps & 5000 \\
     batch size & 256 \\
     utd ratio & 20 \\
     \hline
    \end{tabular}
    \caption{Hyperparameters that are kept constant across all real-world tasks}
    \label{table:realhype1}
\end{table}

\begin{table}[H]
    \centering
    \begin{tabular}{|c ||c |  c |  c |  c|  c |  c |  c |}
    \hline
     & Control & Episode Time & Demo Size & Demo Length & Explore Step & Update  \\
     \hline
     Task / Unit & Hz & s & \# & s & env. steps &  env. steps  \\
     \hline
     \textbf{Reaching} & 8& 6& 15& 4& 1440 & 1440 \\
     \textbf{Pushing} &8 & 6& 15& 4& 1440 & 1440  \\
     \textbf{Obst Pushing} & 8& 12 & 15& 8& 1440 & 1440  \\
     \textbf{Opening} & 8& 10 & 15 & 4& 1440 & 1440  \\
     \textbf{Sweeping} & 8& 12 & 30 &6 & 1440 & 1440  \\
     \textbf{Drawing} & 1 & 16 & 15 & 5& 240 & 240  \\
    \hline
    \end{tabular}
    \caption{Hyperparameters that are varied across each task}
    \label{table:realhype2}
\end{table}
We provide the hyperparameters that we used for the real-world experiments in Table \ref{table:realhype1} and Table \ref{table:realhype2}. Table \ref{table:realhype1} gives the hyperparameters for the methods that were used in the algorithm to run the real-world experiments. If a hyperparameter value was not reported in the table, it is set to \texttt{None} or not used. Table \ref{table:realhype2} provides the hyperparameters used for the training procedure. Notice that our algorithm requires minimal hyperparameter tuning for explorations steps and discriminator updates if the goal is to just have a successful run. This minimum overhead highlights the ease to use of our algorithm for real-world settings. Note that drawing has a drastically different set of hyperparameters because we set the control frequency to 1. Otherwise, the robotic arms would not draw anything reasonable.

\newpage
\subsection{Subsampling Experiment Result}

\begin{table}[!h]
\begin{center}
\begin{tabular}{|| p{2.5 cm} p{1.5 cm} p{1.3 cm} p{1.3 cm} p{1.3 cm} p{1.6 cm} ||}
 \hline
  Task & Reaching & Pushing & Pushing w/ Obst & Drawer Opening & Sweeping \\
 \hline
 Metric & $L2$-dist & $L2$-dist & StS & StS & Incompletion  \\
 \hline\hline
 \Method & 0.31 & 0 & 4391 & 6079 & 0\%  \\
 \Method (w/ subsampling) & 0.29 & 1.26 & 3527 & 4543 & 0\% \\
 \hline
\end{tabular}
\end{center}
\caption{Reaching tasks evaluated with $L2$-distance between the end effector and target position has near identical performance with subsampling during training of the ranking network using our method \Method. All other hyperparameters remained the same as in Table \ref{table:realhype2} under reaching. } 
 \label{table:subsample}
\end{table}

While training from raw videos allows us to utilize an abundance of data, there are some tasks that are inherently hard to demonstrate and therefore lack expert videos. One such example is robotic hand manipulation tasks. It is hard for humans to provide full video demonstrations that could be useful for the agent to learn. However, it is much more reasonable to take multiple pictures across the progression of the task. For instance, a human can adjust the robotic hand, take a picture, adjust it again, and then take another picture. Toward the goal of learning from a few sequential images instead of a full video, we experimented with the reaching task with subsampling of 1 frame per second. Using reaching as example, since the expert video demo length is 4 seconds, we would only have 4 frames per demo to train the reward function as opposed to 32 without subsampling. The demo length of other tasks are provided in Table \ref{table:realhype2}. We found that agents trained with the reward feedback from our \Method perform nearly identically regardless of whether or not subsampling is enabled, as reported in Table \ref{table:subsample}. In some tasks, such as obstacle pushing and drawer opening, subsamplings are even able to successfully complete the task with less training steps. This suggests that \Method could still give quality reward signals even when only a few intermediate snapshots of a task are given, opening up the potential of learning a much wider range of tasks. 

\section{Ego4D Experiments Details}
\subsection{Hyperparameters Tables}
\begin{table}[H]
    \centering
    \begin{tabular}{| c || c |}
     \hline
     \textbf{Data} &  \\
     \hline
     batch size & 32 \\
     epoch & 10 \\
     training data size (frames) & 1.6M \\
     evaluation data size (frames) & 613,660 \\
     \hline
     \textbf{Network} & \\
     \hline
     hidden layers dimensions & 4096 $\times$ 6 layers \\
     non linearity & ReLU \\
     regularization on hidden layers & (None $\times 5$, Spectrual Norm) \\
     \hline
     \textbf{Optimizer} \& \textbf{Scheduler}& \\
     \hline
     optimizer & Adam \\ 
     learning rate & $1 \times 10 ^{-4} $ \\
     scheduler & LinearWarmupConsineAnnealingLR \\
     warmup epoch & 2 \\ 
     maximum epoch & 10 \\ 
     minimum lr & $1 \times 10^{-6}$ \\
     \hline
    \end{tabular}
    \caption{Hyperparameters for Ego4D experiments}
    \label{table:ego4d_hype}
\end{table}
We provide the hyperparamters that we used for training the general ranking function and discrimminator on Ego4D data. Note that the hyperperameters are the same for both.
